# Supplementary material for: Quantum transport in high-quality shallow InSb quantum wells
Source: arXiv:1904.00828 source file (2019-06-25)
Supplement: Supplementary file 1 [file SupplementaryMaterials.pdf]

Supplementary Material to

# Quantum transport in high-quality shallow InSb quantum wells

Zijin Lei*, Christian Lehner, Erik Cheah, Matija Karalic, Christopher Mittag, Luca Alt, Jan Scharnetzky, Werner

Wegscheider, Thomas Ihn, and Klaus Ensslin

*Solid State Physics Laboratory, Department of Physics, ETH Zurich, 8093 Zurich, Switzerland*

*Email: zilei@phys.ethz.ch

## I. Approximate band edge g-factor estimation

We roughly estimate the band edge g-factor like in Ref. 25 of the main text. Based on the saturation of the term $\ln(\Delta\rho_{xx}/\overline{\rho_{xx}})$ at 1.3 K in Fig. 4 (b) of the main text, the thermal contribution of the Landau level broadening $\Gamma$ is insignificant. Beyond the critical field $B_{c1}$, for which the cyclotron energy reaches $\Gamma$, i.e., $\Gamma \approx \hbar e B_{c1}/m^*$, where $m^*$ is the effective mass of electrons in the QW, Shubinikov-de Haas (SdH) oscillations are observed. Similarly, the Zeeman splitting can be observed when the magnetic field exceeds a critical value $B_{c2}$ where the Zeeman energy $\Delta E_Z = \mu_B g B_{c2}$ reaches $\Gamma$. Here, the Bohr magneton $\mu_B = \mathrm{e}\hbar/2\mathrm{m}_0$ . With the assumption that $\Gamma$ is independent of the magnetic field, we obtain the approximate relation $\hbar e B_{c1}/m^* \approx \mu_B g B_{c2}$. Considering that $\nu_{c1} B_{c1} = \nu_{c2} B_{c2}$, where $\nu_{c1}$ and $\nu_{c2}$ are the filling factors corresponding to $B_{c1}$ and $B_{c2}$, and $m^* = 0.019\ m_0$ the band edge g-factor is estimated to be

$$g = \frac{2m_0\nu_{c2}}{m^*\nu_{c1}}.$$

Based on the measurement introduced in the main text, $\nu_{c1} = 16$, $\nu_{c2} = 7$, and $m^* = 0.019\ m_0$. With these values, the absolute value of the band edge g-factor is estimated to be ~ 46.

## II. Magneto-transport characterization of sample 1.

The method used to characterize sample 1 is very similar to that used for sample 2. Figures S1 (a) and (b) show the $\rho_{xx}$ and $\rho_{xy}$ data of sample 1. In Fig. S1 (a), two Landau fan diagrams

are found. The double-fan structure shows that there are two parallel conducting channels in this heterostructure as well. We attribute the first channel to form in the Si doping layer, and the second in the QW layer by virtue of the different gate capacitances obtained from the analysis of *1/B*-periodic SdH oscillations. Fig. S1 (c) shows the corresponding carrier densities $n_1$ (Si layer) and $n_2$ (QW) as a function of $V_{TG}$. In contrast to sample 2, the density of electrons in the QW layer saturates at high $V_{TG} > 0.5$ V. We attribute this saturation to charging of the capping layer in a strong electric field, screening the electric field of the top gate. The two-band Drude model is used to get the mobilities $\mu_1$ and $\mu_2$ of the Si layer and QW layer in sample 1. When the QW layer gets populated, $n_1$ remains roughly constant at a value of $1.4 \times 10^{15}\mathrm{m}^{-2}$ and the mobility $\mu_1$ remains stable at $\mu_1 \sim 8000\ \mathrm{cm}^{-2}(\mathrm{Vs})^{-1}$. The density $n_2$ increases from 0 to $\sim 3.5 \times 10^{15}\mathrm{m}^{-2}$, together with an increase of $\mu_2$ to $\sim 350{,}000\ \mathrm{cm}^{-2}(\mathrm{Vs})^{-1}$ [Fig. S1(d)]. The quality of sample 1 is comparable with the devices in the work by A. M. Gilbertson *et al.* and [1,2], where the upper barrier thickness is also ~50 nm. And the mobility is also higher than the recent report by Ke *et. al.* [3] in a similar QW structure.

Fig. S2 shows the effective mass measurement and the Zeeman splitting in Sample 1. We use the same method introduced in the main text, finding the electron effective mass to be $m^* \approx 0.020\ m_0$. Because the Ando formula is not applicable for large oscillation amplitudes, the calculated effective mass increases when extracted at higher magnetic field. Considering the Zeeman splitting observed in sample 1, we estimate the absolute value of the g-factor to be ~ 50, similar to that in sample 2.

## III. Magneto-transport characterization of sample 3.

Fig. S3 presents the measurement performed on sample 3 and a similar analysis with the previous 2 samples is used. We again find the double-channel structure through $\rho_{xx}$ (Fig. S3 (a)) and $R_{xy}$ (Fig. S3 (b)). The dependence of both Si doping and QW channels on $V_{TG}$ is shown in Fig. S3 (c). When the QW layer gets charged, $n_1$ is roughly constant with a value of $3 \times 10^{15}\mathrm{m}^{-2}$ and the mobility remains at a value $\mu_1 \sim 4000\ \mathrm{cm}^{-2}(\mathrm{Vs})^{-1}$. The density $n_2$ increases from 0 to $\sim 3 \times 10^{15}\mathrm{m}^{-2}$, together with an increase of $\mu_2$ up to $\sim 160{,}000\ \mathrm{cm}^{-2}(\mathrm{Vs})^{-1}$ [Fig. S3 (d)].

## IV. Comparison between Hall bar samples and van der Pauw samples without $Al_2O_3$

There are 3 millimeter-sized van der Pauw (vdP) samples without $Al_2O_3$ and chemical etching fabricated from the same wafers of the 3 Hall bar samples discussed before. The magneto-transport measurements are performed at 1.3 K. Fig. S4 (a) compares sample 1 with $V_{TG} = 0$ V and the corresponding vdP sample. We find that they have similar electron densities in both doping layers and QW. Figs. S4 (b) and (c) shows the comparison between sample 2 and the corresponding vdP sample. Different from sample 1, to get the same carrier density in the vdP sample, where only the doping layer is populated with $n_1 = 2.3 \times 10^{11}\text{cm}^{-2}$ , the top gate voltage should be turned to -0.29 V. As we discussed in the main text, when $V_{\text{TG}} = 0$ V, $n_1$ and $n_2$ are $3.2 \times 10^{11}\text{cm}^{-2}$ and $0.4 \times 10^{11}\text{cm}^{-2}$ in sample 2, respectively. Similarly, to get the same carrier density distribution as its corresponding vdP sample, where $n_1 = 2.5 \times 10^{11}\text{cm}^{-2}$ but $n_2 \approx 0$, $V_{\text{TG}} = -0.36$ V has to be applied on sample 3 [Fig. S4 (d)]. When $V_{\text{TG}} = 0$ V , from the previous analysis, we see that $n_1 = 2.7 \times 10^{11}\text{cm}^{-2}$ and $n_2 = 2.2 \times 10^{11}\text{cm}^{-2}$ in sample 3 [Fig. S4 (e)]. We attribute the $V_{\text{TG}}$ shift in the wafers without InSb capping layer to a positive residual charge present after deposition of insulator and gate-metal. The lower mobility in Hall bar samples may be due to sample aging.

## V. Band structure simulation on sample 1 and sample 2

We used the commercial software Nextnano [4] to perform self-consistent Schrödinger-Poisson simulations on sample 1 and sample 2 neglecting the ALO dielectric layers. Here, carrier densities, wave functions and band structures are presented as a function of growth direction $Z$, where $Z = 0$ correspond to the sample surface. A constant electric field on the substrate side serves as the boundary condition. The doping level in the simulation is taken to be the same as the nominal doping density incorporated during the MBE growth, which is $\sim 3 \times 10^{12}\text{cm}^{-2}$. As shown in Fig. S5 (a), for sample 1, when the bias voltage on the sample surface $V_{\text{bias}} = 0$, both the Si-doping layer and the QW are populated with electrons. Increasing $V_{\text{bias}}$ to 0.3 V, the electron density in the QW increases more significantly than the electron density in the Si-doping layer. Fig. S5 (b) presents the dependences of the electron densities $n_1$ and $n_2$ in Si-doping layer and QW on $V_{\text{bias}}$, respectively. When electrons populate the QW, the increase of $n_1$ slows down due to screening, in agreement with the experiment in the main text. The saturation of $n_2$ at high $V_{\text{bias}}$ is due to electrons populating the InSb capping layer. The wave function of electrons in the capping layer is shown with the pink dashed line. The situation in sample 2 is similar and presented in Fig. S5 (c) and (d). Electrons populate the Si-doping layer at $V_{\text{bias}} = 0$ and there is no saturation of $n_2$ at high $V_{\text{bias}}$.

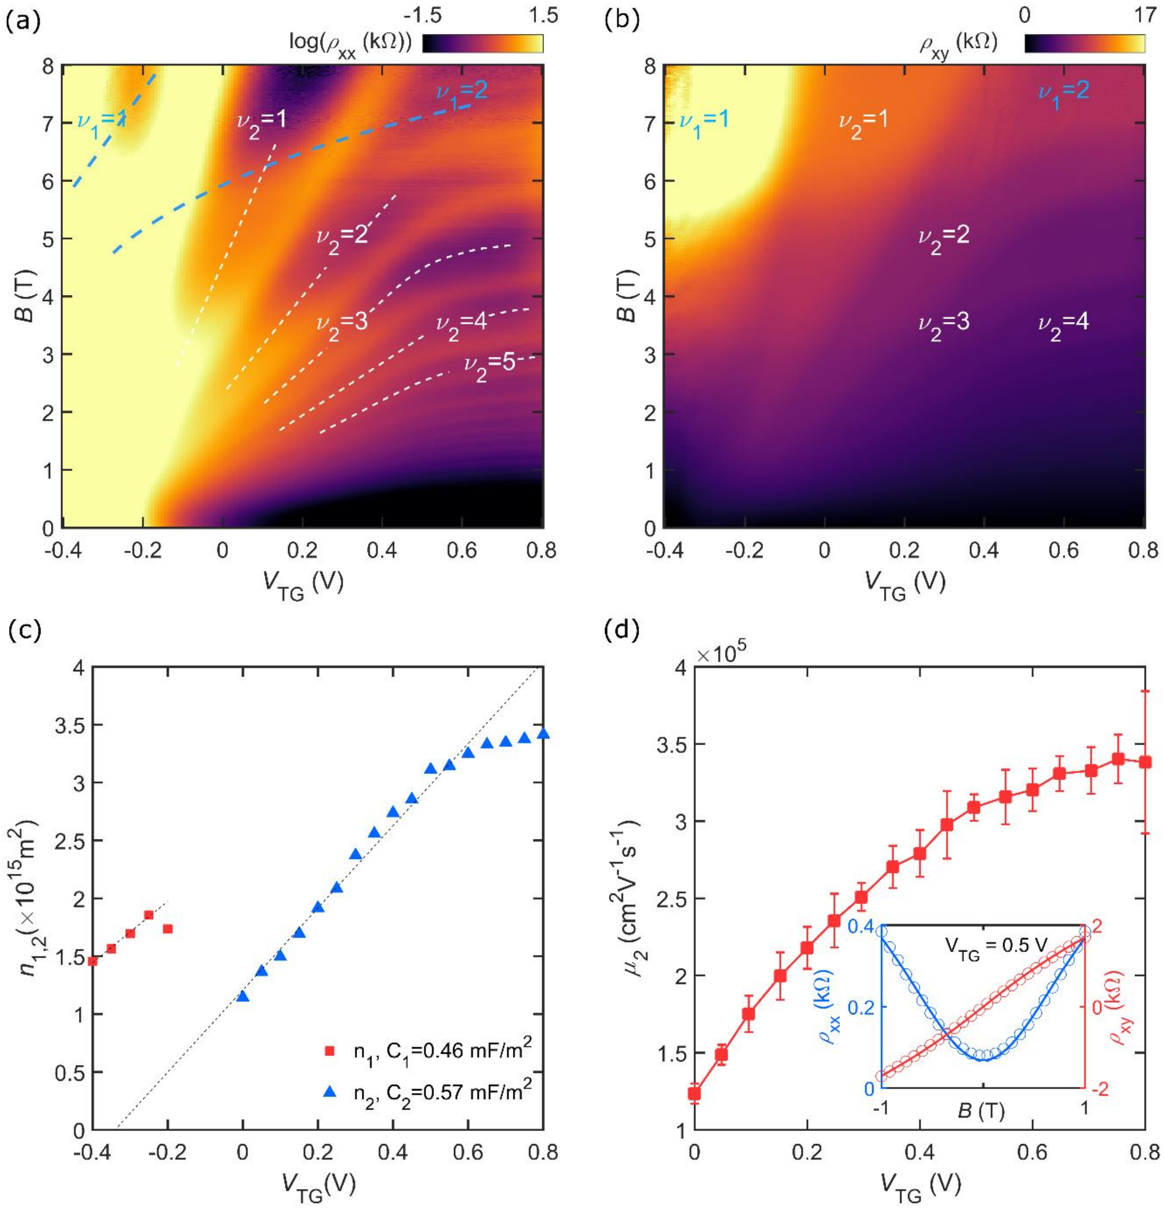


Fig. S1. Magneto-transport characterization performed on sample 1 at 1.7 K. The $V_{TG}$ and $B$ dependence of $R_{xx}$ (a) and $R_{xy}$ (b). The Landau fan diagrams and filling factors of the electrons in the doping layer and the QW layer are labeled with blue and white dashed lines, respectively. (c) Carrier densities of two conductive channels vs. $V_{TG}$. The gate capacitance $C_1$ and $C_2$ show that the Si layer and the QW layer get charged one after another. (d) The mobility of electrons in QW $\mu_2$ vs. $V_{TG}$. Insert: the data (circles) and fitting (lines) of $\rho_{xx}$ (red) and $\rho_{xy}$ (blue) vs. $B$ when $V_{TG} = 0.5$ V.

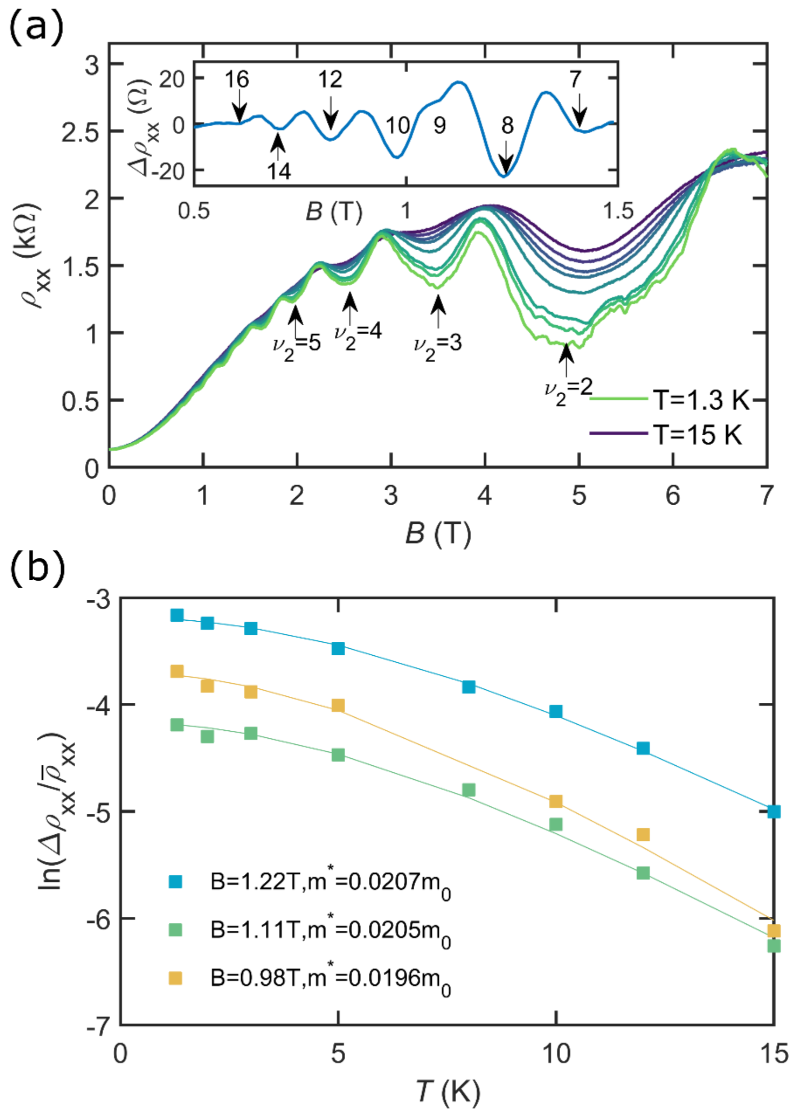


Fig. S2. Effective mass measurement and the Zeeman splitting of Sample 2. (a) Temperature dependence of SdH oscillations. Insert: $\Delta\rho_{xx}$ in a small magnetic field. The Zeeman splitting happens at around $\nu_2 = 9$. (b) Dingle factor fitting with different $B$. The squares are data and the lines are fitted curves.

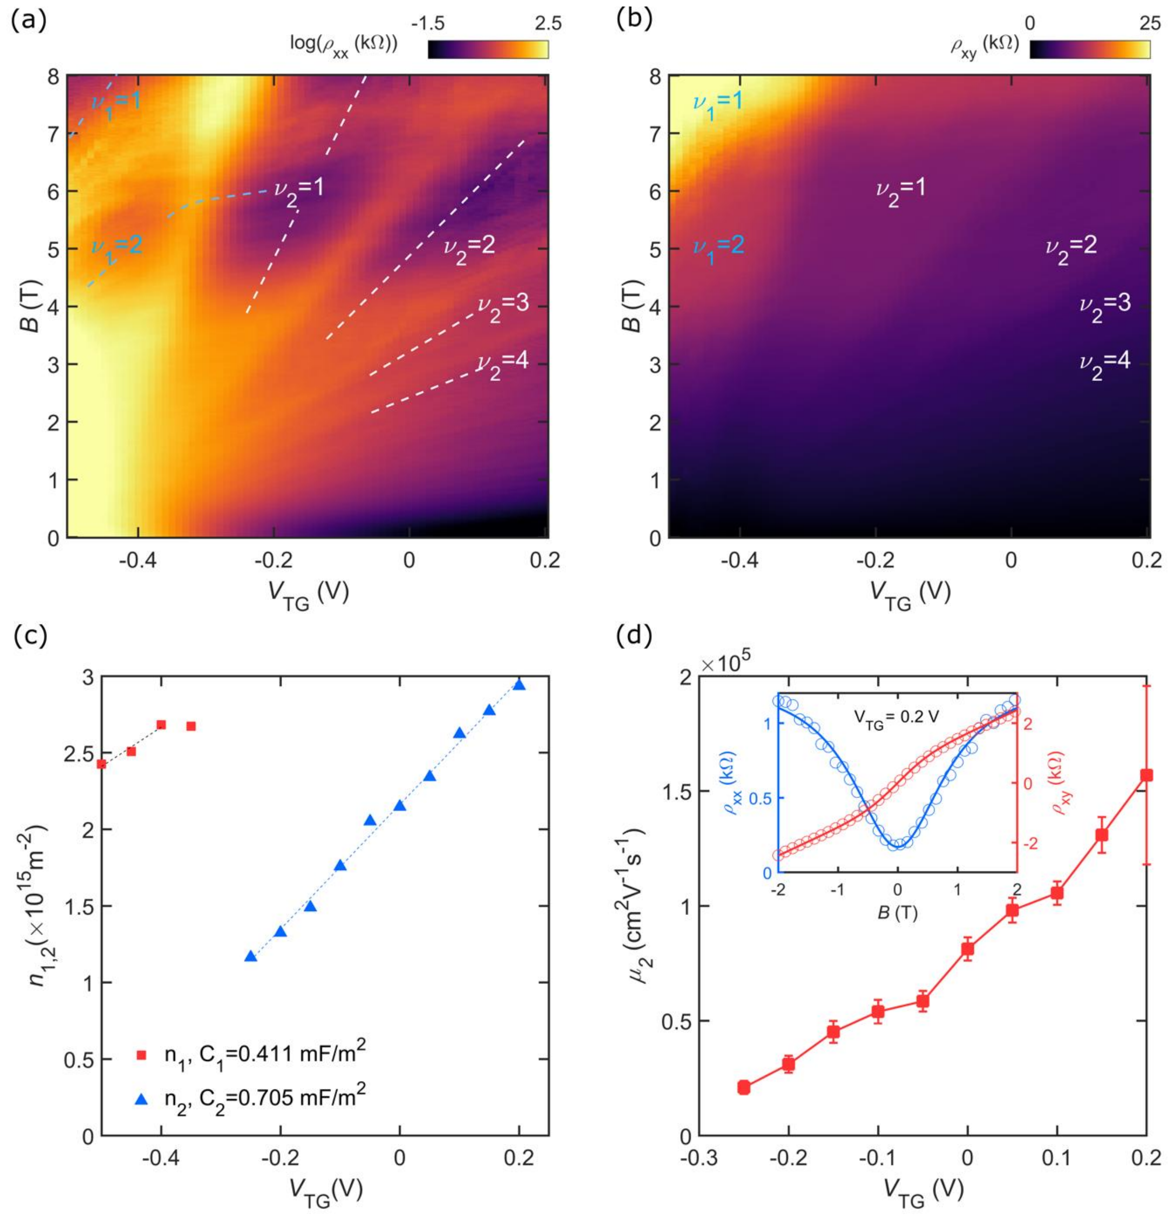


Fig. S3. Magneto-transport characterization performed on sample 3 at 1.7 K. The $V_{TG}$ and $B$ dependence of $\rho_{xx}$ (a) and $\rho_{xy}$ (b). (c) Carrier densities of two conductive channels vs. $V_{TG}$. (d) The mobility of electrons in QW $\mu_2$ vs. $V_{TG}$. Insert: the data (circles) and fitting (lines) of $\rho_{xx}$ (red) and $\rho_{xy}$ (blue) vs. $B$ when $V_{TG} = 0.2$ V.

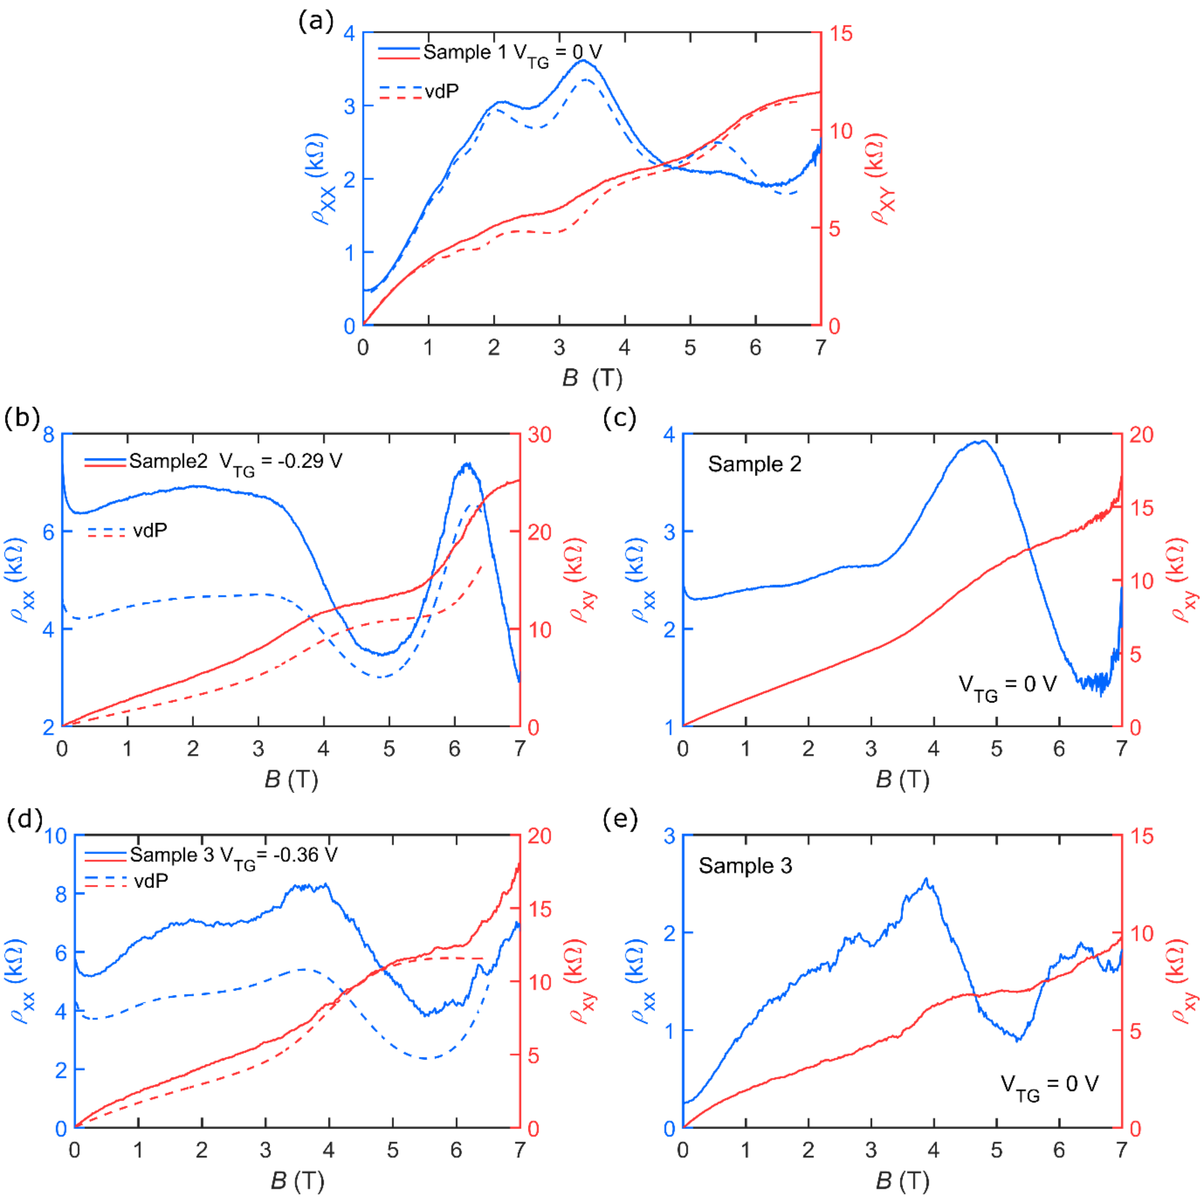


Fig. S4. (a) Magneto-transport measurement of sample 1 with $V_{TG} = 0$ and the corresponding vdP sample. (b)(c) Comparison of sample 2 with the corresponding vdP sample. (d)(e) Comparison of sample 3 with the corresponding vdP sample.

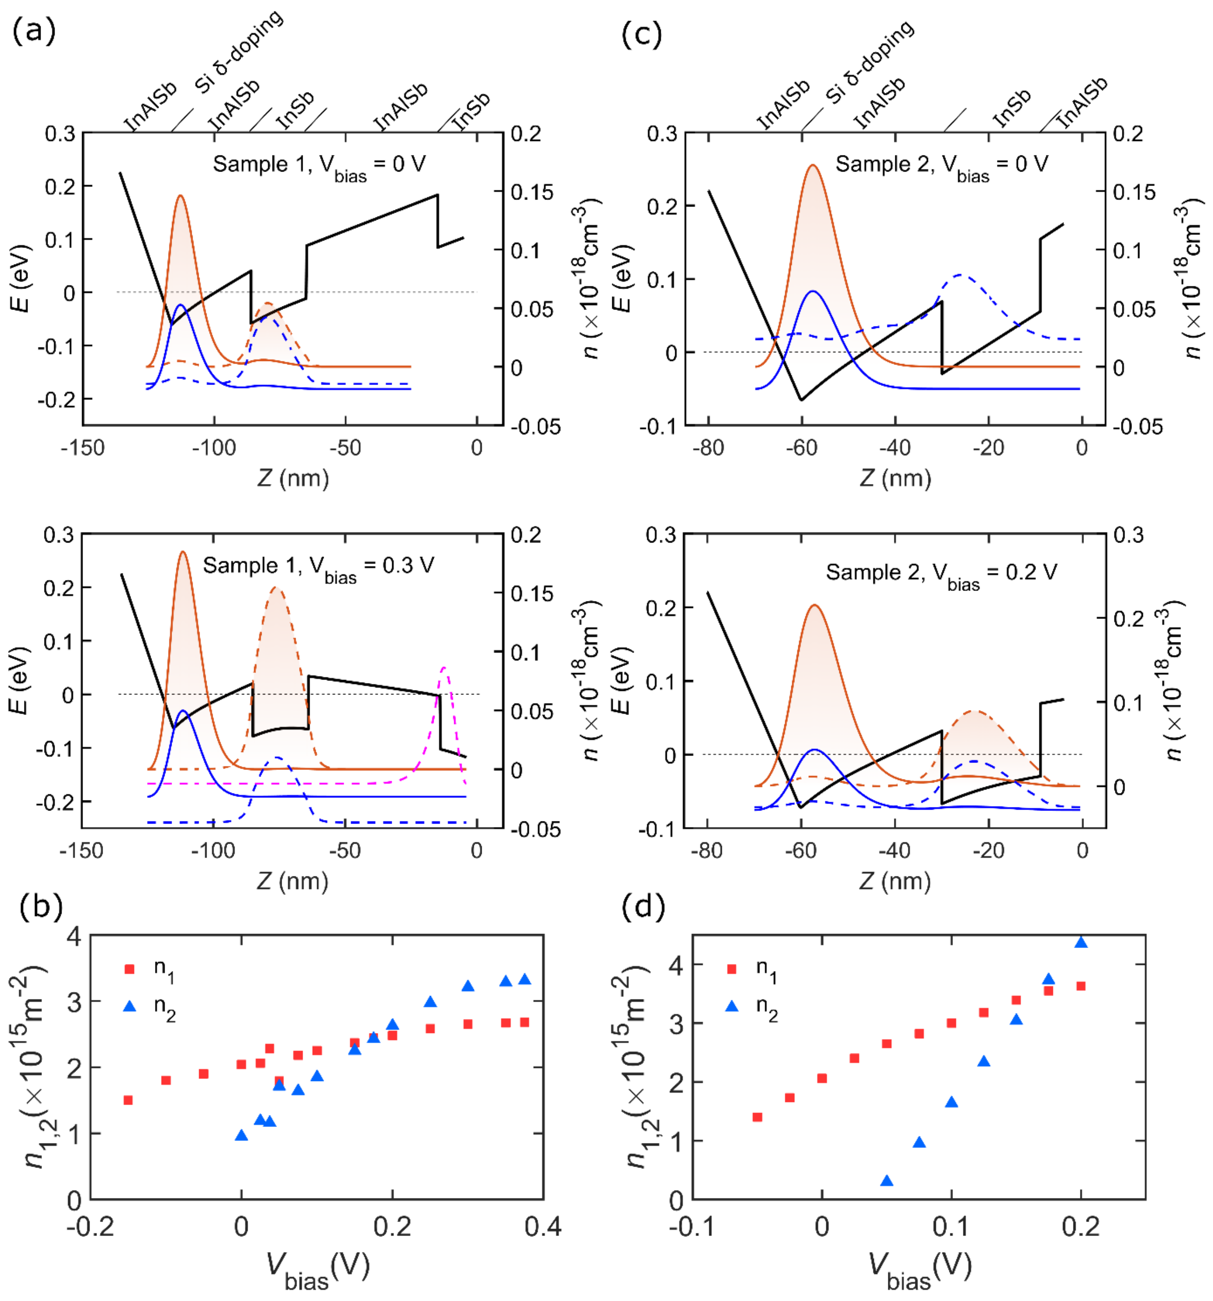


Fig. S5. Simulation results of sample 1 [(a) and (b)] and sample 2[(c)and (d)]. (a) The simulation results of sample 1 where $V_{\text{bias}}$ is set to be 0 V and 0.3 V. (b) The carrier densities in Si-doping layer ($n_1$) and QW ($n_2$) of sample 1 vs. $V_{\text{bias}}$. (c) The simulation results of sample 2 where $V_{\text{bias}}$ is set to be 0 V and 0.2 V. (d) The carrier densities in Si-doping layer ($n_1$) and QW ($n_2$) of sample 2 vs. $V_{\text{bias}}$. In (a) and (c), the thick black lines depict the conduction bands. The solid (dashed) orange lines show the carrier densities of electrons in Si-doping layer (QW). Solid (dashed) blue lines are the wave functions of electrons in Si-doping layer (QW). The pink dashed line in (a) is the wave function of electrons in the InSb capping layer. The Fermi level is presented as the dashed black lines.

## References

[1] A. M. Gilbertson, W. R. Branford, M. Fearn, L. Buckle, P. D. Buckle, T. Ashley, and L. F. Cohen, "Zero-field spin splitting and spin-dependent broadening in high-mobility InSb/In1−xAlxSb asymmetric quantum well heterostructures", Phys. Rev. B **79**, 235333 (2009)

[2] Wei Yi1, Andrey A. Kiselev, Jacob Thorp, Ramsey Noah, Binh-Minh Nguyen, Steven Bui, Rajesh D. Rajavel, Tahir Hussain, Mark F. Gyure, Philip Kratz, Qi Qian, Michael J. Manfra, Vlad S. Pribiag, Leo P. Kouwenhoven, Charles M. Marcus, and Marko Sokolich, "Gate-tunable high mobility remote-doped $InSb/In_{1-x}Al_xSb$ quantum well heterostructures", Appl. Phys. Lett. **106**, 142103 (2015)

[3] Chung Ting Ke, Christian M. Moehle, Folkert K. de Vries, Candice Thomas, Sara Metti, Charles R. Guinn, Ray Kallaher, Mario Lodari, Giordano Scappucci, Tiantian Wang, Rosa E. Diaz, Geoffrey C. Gardner, Michael J. Manfra, Srijit Goswami, "Ballistic superconductivity and tunable $\pi$-junctions in InSb quantum wells", arXiv:1902.10742

[4] S. Birner, T. Zibold, T. Andlauer, T. Kubis, M. Sabathil, A. Trellakis, P. Vogl, "General Purpose 3-D Simulations", IEEE Trans. Electron Dev. **54**, 2137 (2007)
